# Supplementary material for: Polynomial Neural Fields for Subband Decomposition and Manipulation
Source: arXiv:2302.04862 source file (2023-02-09)
Supplement: Supplementary file 1 [file fig.tex]

\newcolumntype{Y}{>{\centering\arraybackslash}X}
\begin{figure*}
\begin{center}
\begin{tabular}{c@{}c@{}c@{}c@{~~~}c@{}c@{}c@{}c@{}c}
\includegraphics[width=0.12\linewidth,height=0.12\linewidth]{figures/laplacian_supp2/bacon/05_BACON_log_quant_last_gau_0.png} &
\includegraphics[width=0.12\linewidth,height=0.12\linewidth]{figures/laplacian_supp2/bacon/05_BACON_log_quant_last_lap_1.png} &
\includegraphics[width=0.12\linewidth,height=0.12\linewidth]{figures/laplacian_supp2/bacon/05_BACON_log_quant_last_lap_2.png} &
\includegraphics[width=0.12\linewidth,height=0.12\linewidth]{figures/laplacian_supp2/bacon/05_BACON_log_quant_last_lap_3.png} &
\includegraphics[width=0.12\linewidth,height=0.12\linewidth]{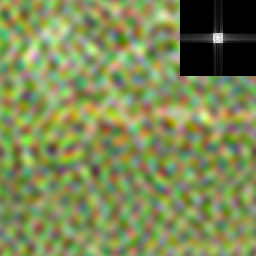} &
\includegraphics[width=0.12\linewidth,height=0.12\linewidth]{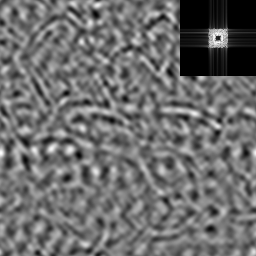} &
\includegraphics[width=0.12\linewidth,height=0.12\linewidth]{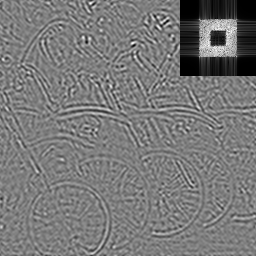} &
\includegraphics[width=0.12\linewidth,height=0.12\linewidth]{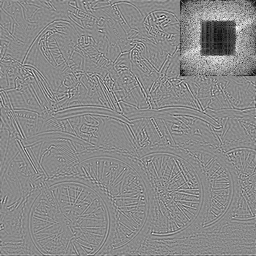} \\

\includegraphics[width=0.12\linewidth,height=0.12\linewidth]{figures/laplacian_supp2/bacon/05_BACON_log_quant_last_gau_0.png} &
\includegraphics[width=0.12\linewidth,height=0.12\linewidth]{figures/laplacian_supp2/bacon/05_BACON_log_quant_last_gau_1.png} &
\includegraphics[width=0.12\linewidth,height=0.12\linewidth]{figures/laplacian_supp2/bacon/05_BACON_log_quant_last_gau_2.png} &
\includegraphics[width=0.12\linewidth,height=0.12\linewidth]{figures/laplacian_supp2/bacon/05_BACON_log_quant_last_gau_3.png} &
\includegraphics[width=0.12\linewidth,height=0.12\linewidth]{figures/laplacian_supp2/pnf/05_pnf_PNF_pseudopolar_fix2_gau_0.png} &
\includegraphics[width=0.12\linewidth,height=0.12\linewidth]{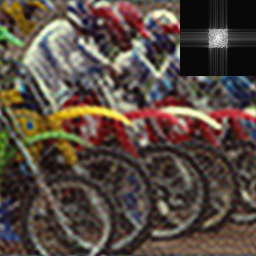} &
\includegraphics[width=0.12\linewidth,height=0.12\linewidth]{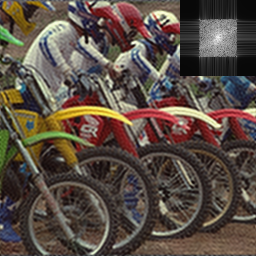} &
\includegraphics[width=0.12\linewidth,height=0.12\linewidth]{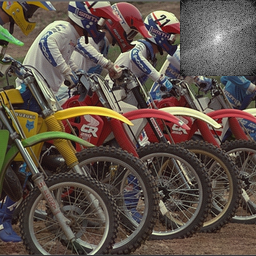}
 \\
 \multicolumn{4}{c}{BACON} & \multicolumn{4}{c}{PNF}
\end{tabular}
\caption{BACON: The bottom row shows the output of each layer which is upper band limited. The top row (columns 2-4) shows the difference between the output of a given layer and the one before it. PNF: The top row shows the output of each layer which is both upper and lower band limited. The bottom row (columns 2-4) shows the addition of the output at a given layer and the one before it. }
\label{fig:laplacian-pyramid_supp2}
\end{center}
\end{figure*}
